# Supplementary material for: Greedy Network Enlarging
Source: arXiv:2108.00177 source file (2021-11-26)
Supplement: Supplementary file 2 [file appendix.pdf]

## A Appendix

### A.1 Performance Estimation

#### A.1.1 Proxy dataset

For the proxy sub-dataset, we create two sub-datasets ImageNet1000-100 and ImageNet100-500 by random selecting images from ImageNet [2]. ImageNet1000-100 has 1000 classes and each class has 100 images, while ImageNet100-500 has 100 classes and each class has 500 images. The validation set of ImageNet1000-100 is the original validation dataset with 50K images. The validation set of ImageNet100-500 is the sub-dataset of ImageNet validation set, it contains the selected 100 categories and 5K images.

| Model | input size | depth         | width                    | Top-1 |
|-------|------------|---------------|--------------------------|-------|
| a1    | 224        | 3,2,2,3,3,4,1 | 16,24,40,80,112,192,320  | 75.62 |
| a2    | 224        | 1,4,2,3,3,4,1 | 16,24,40,80,112,192,320  | 75.96 |
| a3    | 224        | 1,2,4,3,3,4,1 | 16,24,40,80,112,192,320  | 75.90 |
| a4    | 224        | 1,2,2,4,4,4,1 | 16,24,40,80,112,192,320  | 76.02 |
| a5    | 224        | 1,2,2,3,3,6,1 | 16,24,40,80,112,192,320  | 76.14 |
| a6    | 224        | 1,2,2,3,3,4,1 | 24,24,40,80,112,192,320  | 75.77 |
| a7    | 224        | 1,2,2,3,3,4,1 | 16,36,40,80,112,192,320  | 75.78 |
| a8    | 224        | 1,2,2,3,3,4,1 | 16,24,60,80,112,192,320  | 76.06 |
| a9    | 224        | 1,2,2,3,3,4,1 | 16,24,40,100,140,192,320 | 76.41 |
| a10   | 224        | 1,2,2,3,3,4,1 | 16,24,40,80,112,224,364  | 76.33 |
| a11   | 240        | 1,2,2,3,3,4,1 | 16,24,40,80,112,192,320  | 76.22 |
| a12   | 256        | 1,2,2,3,3,4,1 | 16,24,40,80,112,192,320  | 76.55 |

Table 1: 12 network architectures with different input size, width and depth. Their Top-1 accuracies on ImageNet for train 150 epochs are shown.

To evaluate these datasets, 12 network architectures 1 with different width, depth and input sizes are generated on the basis of EfficientNet-B0 [3]. We train all the 12 networks on the whole train set of ImageNet for 150 epochs, the Top-1 accuracies on the validation dataset are used as the comparison object.

The finetune method comes from function preserving algorithm [1]. The weight transfer method rapidly transfers knowledge from the previous best model into each new model that an experimenter proposes.

On EfficientNet-B0, we train two models with ImageNet1000-100 and ImageNet100-500 for 150 epochs, respectively. For each dataset, we finetune the 12 networks for 5, 10 and 20 epochs on the basis of pretrained models, and train the 12 networks from scratch for 10 and 20 epochs. 2 random seed 0 and 42 are used. Totally, we have  $2 \times 2 \times 2 \times (3 + 2) \times 12 = 480$  evaluation results. On ImageNet100-500, the average Spearman value is  $\rho = 0.16$ . On ImageNet1000-100, the average Spearman value is  $\rho = 0.23$ . So we choose ImageNet1000-100 as the proxy sub-dataset. The accuracies of all configurations are in the excel sheets named with proxy\_dataset.xlsx.

#### A.1.2 Search hyper-parameters

The correlation between the proxy task and original task is not significant according to the previous section. By adjusting the hyper-parameters of training, the result will be more stable and the correlation will be improved. 12 new network architectures 2 with different width, depth and input sizes are created on the basis of EfficientNet-B0. Together with previous 12 architectures, we make experiments on 24 networks.

| Model | input size | depth         | width                   | Top-1 |
|-------|------------|---------------|-------------------------|-------|
| a13   | 224        | 2,3,2,3,3,4,1 | 16,24,40,80,112,192,320 | 75.95 |
| a14   | 224        | 1,3,2,3,3,4,1 | 16,24,40,80,112,192,320 | 75.84 |
| a15   | 224        | 1,2,3,3,3,4,1 | 16,24,40,80,112,192,320 | 75.72 |
| a16   | 224        | 1,2,2,4,3,4,1 | 16,24,40,80,112,192,320 | 75.87 |
| a17   | 224        | 1,2,2,3,3,5,1 | 16,24,40,80,112,192,320 | 76.04 |
| a18   | 224        | 1,2,2,3,3,4,1 | 20,24,40,80,112,192,320 | 75.67 |
| a19   | 224        | 1,2,2,3,3,4,1 | 16,28,40,80,112,192,320 | 75.81 |
| a20   | 224        | 1,2,2,3,3,4,1 | 16,24,50,80,112,192,320 | 75.89 |
| a21   | 224        | 1,2,2,3,3,4,1 | 16,24,40,90,124,192,320 | 75.90 |
| a22   | 224        | 1,2,2,3,3,4,1 | 16,24,40,80,112,208,344 | 75.84 |
| a23   | 224        | 1,2,2,3,4,4,1 | 16,24,40,80,112,192,320 | 75.91 |
| a24   | 224        | 1,2,2,3,3,4,2 | 16,24,40,80,112,192,320 | 76.28 |

Table 2: Another 12 network architectures. Their Top-1 accuracies on ImageNet for train 150 epochs are shown.

We train all of the 24 networks on the whole train set of ImageNet for 150 epochs, the Top-1 accuracies on the validation dataset are used as the comparison object. Two pretrained EfficientNet-B0 models on the ImageNet and ImageNet1000-100 are provided, respectively. Besides, the learning rate is 0.01 and 0.002 for finetuning and 0.1 for training from scratch. The learning rate decay mode is selected from cosine and multi-step. All models are trained for 10 and 20 epochs, respectively. The trick of model ema (exponential moving average) is used. For training from scratch, we test 10 hyper-parameter combinations. For finetuning, 32 hyper-parameter combinations are tested. Totally, there are  $42 * 24 = 1008$  network architectures are evaluated. Among these 42 hyper-parameter settings, the top-2 Spearman value  $\rho$  is 0.57 and 0.54, these values indicate moderate positive correlation. They both use cosine decay method and the initial learning rate is 0.01 for training 20 epochs. The difference is that the first use the ImageNet1000-100 pretrained model and the second use the ImageNet pretrained model. The accuracies of all configurations are in the excel sheets named with hyper-parameter.xlsx. In the section of experiments, we take use of initial learning rate is 0.01 and cosine decay for finetuning 20 epochs on the ImageNet1000-100 pretrained model.

## A.2 Experiment results

In this section, we release all searched model architectures 3 including S-EfficientNet and S-GhostNet.

| Model             | input size | depth          | width                   | Top-1(%) | Top-5(%) |
|-------------------|------------|----------------|-------------------------|----------|----------|
| S-EfficientNet-B1 | 256        | 1,2,2,3,3,10,1 | 16,24,40,80,112,192,320 | 79.91    | 94.81    |
| S-EfficientNet-B2 | 288        | 1,2,2,4,5,10,1 | 16,24,40,80,112,192,320 | 80.92    | 95.28    |
| S-EfficientNet-B3 | 304        | 2,3,4,6,6,10,1 | 22,32,50,86,120,220,366 | 81.98    | 95.79    |
| S-EfficientNet-B4 | 384        | 2,4,4,6,8,12,1 | 24,40,64,94,132,240,400 | 83.00    | 96.06    |
| S-GhostNet-B1     | 248        | 3,2,5,12,2,11  | 24,24,64,100,140,280    | 80.08    | 94.82    |
| S-GhostNet-B4     | 384        | 3,4,5,10,8,14  | 28,56,108,164,228,336   | 83.23    | 96.26    |

Table 3: Searched architectures.

## References

- [1] Tianqi Chen, Ian Goodfellow, and Jonathon Shlens. Net2net: Accelerating learning via knowledge transfer. *arXiv preprint arXiv:1511.05641*, 2015.

- 49 [2] Jia Deng, Wei Dong, Richard Socher, Li-Jia Li, Kai Li, and Fei-Fei Li. Imagenet: A large-scale  
50 hierarchical image database. In *CVPR*, 2009.
- 51 [3] Mingxing Tan and Quoc V Le. Efficientnet: Rethinking model scaling for convolutional neural  
52 networks. *arXiv preprint arXiv:1905.11946*, 2019.
